# Supplementary material for: The Effect of Masking Strategies on Knowledge Retention by Language Models
Source: arXiv:2306.07185 source file (2023-06-12)
Supplement: Supplementary file 1 [file appendix.tex]

\section{Appendix}
